# Supplementary material for: Ultra-relativistic electron beams deflection by quasi-mosaic crystals
Source: arXiv:2110.12959 source file (2022-01-25)
Supplement: Supplementary file 1 [file SM_for_qmBC_RPL.pdf]

# Supplemental Material for "Ultra-relativistic electron beams deflection by quasi-mosaic crystals"

Gennady B. Sushko,[1,*] Andrei V. Korol,[1,†] and Andrey V. Solov'yov[1,‡]

[1] *MBN Research Center, Altenhöferallee 3, 60438 Frankfurt am Main, Germany*

## Abstract

In what follows some explanatory material, additional to the main text, is presented.

## METHODS FOR MANUFACTURING OF BENT CRYSTALS

Approaches that have been utilised to produce bent crystals include mechanical scratching [1], laser ablation technique [2], grooving method [3, 4], tensile/compressive strips deposition [3, 5, 6], ion implantation [7]. The most recent techniques proposed are based on sandblasting one of the major sides of a crystal to produce an amorphized layer capable of keeping the sample bent [8] and on pulsed laser melting processing that produces localized and high-quality stressing alloys on the crystal surface [9].

To increase the bending curvature one can rely on production of graded composition strained layers in an epitaxially grown $Si_{1-x}Ge_x$ superlattice [10, 11]. Both silicon and germanium crystals have the diamond structure with close lattice constants. Replacement of a fraction of Si atoms with Ge atoms leads to bending crystalline directions. By means of this method sets of periodically bent crystals have been produced and used in channeling experiments [12]. A similar effect can be achieved by graded doping during synthesis to produce diamond superlattice [13]. Both boron and nitrogen are soluble in diamond, however, higher concentrations of boron can be achieved before extended defects appear [13, 14]. The advantage of a diamond crystal is radiation hardness allowing it to maintain the lattice integrity in the environment of very intensive beams [15].

## RANGES OF PARAMETERS CONSISTENT WITH THE CHANNELING CONDITION

Figure S1 illustrates the dependences discussed in connection with Eqs. (1)-(5) of the main text. The lines and symbols presented refer to the crystal thickness $L = 60$ $\mu$m and Lindhard's critical angle $\theta_{\rm L} = 80$ $\mu$rad.

The lower solid (green) line shows the linear dependence of the coordinate $h_0$, which corresponds to the zero entrance angle $\theta_e = 0$, with the anticlastic radius $R_{\rm a}$. In this case, the deflection angle $\theta_s$ of a particle accepted at the entrance and channeled through the whole crystal is equal to 400 $\mu$rad. The upper (red) line indicates the values of the transverse coordinate $h$ that are displaced from $h_0$ by the distance $\Delta h_{\max} = \theta_{\rm L} R_{\rm a}$, see Eq. (4). If at the crystal entrance the transverse coordinate exceeds $h_0 + \Delta h_{\max}$ then such a particle, most probable, will not be captured in the channeling regime. The dashed line corresponds to

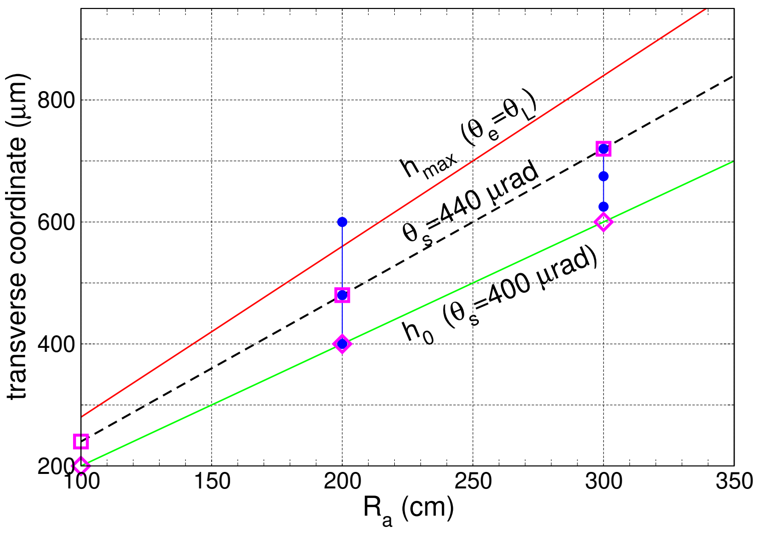


FIG. S1. Dependences of $h_0$ and $h_0 + \Delta h_{\max}$ (solid lines) as functions of the anticlastic curvature radius. Dashed line shows the transverse coordinate at the entrance that provides the deflection angle of 0.44 mrad for channeling particles.

the initial transverse coordinates which result in the deflection angle $\theta_s = 0.44$ $\mu$rad for the channeling particles.

Open rectangles and diamonds indicate the $R_{\rm a}$ and $h$ values that correspond to the data presented in Figure 2 of the main text.

Vertical (blue) lines with symbols indicate the values of $R_{\rm a}$ and coordinates $h$ (closed circles) that have been used in the simulations presented in Figure 3 of the main text.

## GEOMETRY ANALYSIS FOR THE VOLUME CAPTURE AND REFLECTION REGIMES

Particles entering the crystal in the region $\Delta h < 0$ can experience either the volume capture [16] or the volume reflection [17] of the curved crystalline planes during their propagation through the crystal volume. These events take place at the points in space at which the particles trajectories become tangent to the crystalline planes. This condition is fulfilled for most of the particle trajectories entering the crystal at distances $-h_0 < h < h_0$. with respect to the central line corresponding to $h = 0$. For a given $h$ the point of the volume capture and the volume reflection is positioned at the distance $L/2 - R_{\rm qm}h/R$ from the particle entrance point to the crystal. Thus this distance is equal to zero at $h = h_0$ and to

$L$ at $h = -h_0$. Particles moving in the channeling regime after the volume capture exit the crystal at

$$\theta_{\rm s}^{\rm vc}(h) = \theta_{\rm e}(h) + \frac{\theta_{\rm qm}}{2} + \frac{h}{R} \tag{S1}$$

In the process of volume reflection particles are deflected on the characteristic angle $\theta_{vr}$ which does not depend on the choice of $h$ and the location of the volume reflection event in space. The angle $\theta_{vr}$ is determined by the radius $R_{\rm qm}$ and the particle energy. After the volume reflection particles experience multiple scattering within the remaining crystal volume and exit the crystal at the characteristic angle

$$\theta_{\rm s}^{\rm vr}(h) = \theta_{\rm vr} \tag{S2}$$

---


* sushko@mbnexplorer.com

† korol@mbnexplorer.com; On leave from: St. Petersburg State Marine Technical University, Leninsky ave. 101, 198262 St. Petersburg, Russia

‡ solovyov@mbnresearch.com; On leave from: Ioffe Physical-Technical Institute, Politekhnicheskaya 26, 194021 St. Petersburg, Russia



[1] S. Bellucci, S. Bini, V. M. Biryukov, Yu. A. Chesnokov, et al. *Experimental study for the feasibility of a crystalline undulator.* Phys. Rev. Lett. **90**, 034801 (2003).

[2] P. Balling, J. Esberg, K. Kirsebom, D. Q. S. Le, U. I. Uggerhøj, S. H. Connell, J. Härtwig, F. Masiello, and A. Rommeveaux. *Bending diamonds by femto-second laser ablation.* Nucl. Instrum Meth. B **267**, 2952 (2009).

[3] V. Guidi, A. Antonioni, S. Baricordi, F. Logallo, C. Malagù, E. Milan, A. Ronzoni, M. Stefancich, G. Martinelli, and A. Vomiero. *Tailoring of silicon crystals for relativistic-particle channeling.* Nucl. Instrum. Meth. B **234**, 40 (2005).

[4] E. Bagli, L. Bandiera, V. Bellucci, A. Berra, R. Camattari, D. De Salvador, G. Germogli, V. Guidi, L. Lanzoni, D. Lietti, A. Mazzolari, M. Prest, V. V. Tikhomirov, and E. Valla. *Experimental evidence of planar channeling in a periodically bent crystal.* Eur. Phys. J. C **74**, 3114 (2014).

[5] V. Guidi, A. Mazzolari, G. Martinelli, and A. Tralli. *Design of a crystalline undulator based on patterning by tensile $Si_3N_4$ strips on a Si crystal.* Appl. Phys. Lett. **90**, 114107 (2007).

[6] V. Guidi, L. Lanzoni, and A. Mazzolari. *Patterning and modeling of mechanically bent silicon plates deformed through coactive stresses.* Thin Solid Films **520**, 1074 (2011).

[7] V. Bellucci, R. Camattari, V. Guidi, A. Mazzolari, G. Paterno, G. Mattei, C., Scian, and L. Lanzoni. *Ion implantation for manufacturing bent and periodically bent crystals.* Appl. Phys. Lett. **107**, 064102 (2015).

[8] R. Camattari, G. Paternò, M. Romagnoni, V. Bellucci, A. Mazzolari and V. Guidi. *Homogeneous self-standing curved monocrystals, obtained using sandblasting, to be used as manipulators of hard X-rays and charged particle beams.* J. Appl. Cryst. **50** (2017) 145-151.

[9] F. Cristiano, M. Shayesteh, R. Duffy, K. Huet, F. Mazzamuto, Y. Qiu, M. Quillec, H. H. Henrichsen, P. F. Nielsen, D. H. Petersen, A. La Magna, G. Caruso, and S. Boninelli. *Defect evolution and dopant activation in laser annealed Si and Ge.* Mat. Scie. in Semicond. Process. **42** (2016) 188-195

[10] S. A. Bogacz and J. B. Ketterson. *Possibility of obtaining coherent radiation from a solid state undulator.* J. Appl. Phys. **60**, 177 (1986).

[11] U. Mikkelsen and E. Uggerhøj. *A crystalline undulator based on graded composition strained layers in a superlattice.* Nucl. Instum. Meth. B **160**, 435 (2000).

[12] H. Backe, D. Krambrich, W. Lauth, K. K. Andersen, J. L. Hansen, and U. I. Uggerhøj. *Radiation emission at channeling of electrons in a strained layer* $Si_{1-x}Ge_x$ *undulator crystal.* Nucl. Instum. Meth. B **309**, 37 (2013).

[13] T. N. Tran Thi, J. Morse, D. Caliste, B. Fernandez, D. Eon, J. Härtwig, C. Barbay, C. Mer-Calfati, N. Tranchant, J. C. Arnault, T. A. Lafford, and J. Baruchel. *Synchrotron Bragg diffraction imaging characterization of synthetic diamond crystals for optical and electronic power device applications.* J. Appl. Cryst. **50**, 561 (2017).

[14] B. G. de la Mata, A. Sanz-Hervás, M. G. Dowsett, M. Schwitters, and D. Twitchen. *Calibration of boron concentration in CVD single crystal diamond combining ultralow energy secondary ions mass spectrometry and high resolution X-ray diffraction.* Diamond and Rel. Mat. **16**, 809 (2007).

[15] U. Uggerhøj. *The interaction of relativistic particles with strong crystalline fields.* Rev. Mod. Phys. **77**, 1131 (2005).

[16] A. M. Taratin and S. A. Vorobiev. *"Volume trapping" of protons in the channeling regime in a bent crystal.* Phys. Lett. **115**, 398 (1986).

[17] A. M. Taratin and S. A. Vorobiev. *Volume reflection of high-energy charged particles in quasi-channeling states in bent crystals.* Phys. Lett. **119**, 425 (1987).

[18] U. Wienands, T. W. Markiewicz, J. Nelson, R. J. Noble, J. L. Turner, U. I. Uggerhøj, T. N. Wistisen, E. Bagli, L. Bandiera, G. Germogli, V. Guidi, A. Mazzolari, R. Holtzapple, and M. Miller. *Observation of deflection of a beam of multi-GeV electrons by a thin crystal.* Phys. Rev. Let. **114**, 074801 (2015).
